# Supplementary material for: Worldwide spreading of economic crisis
Source: arXiv:1008.3893 source file (2010-08-23)
Supplement: Supplementary file 1 [file SupplementaryInformation-GarasArgyrakisRozenblatTomassiniHavlin.pdf]

# Worldwide spreading of economic crisis

# Supplementary Information

A. Garas[1], P. Argyrakis[1], C. Rozenblat[2], M. Tomassini[3] & S. Havlin[4]

[1]Department of Physics, University of Thessaloniki, 54124 Thessaloniki Greece, GR.

[2]Geography Institute, Faculty of Geosciences, University of Lausanne, 1015 Lausanne Switzerland, CH.

[3]Faculty of Business and Economics, University of Lausanne, 1015 Lausanne Switzerland, CH.

[4]Minerva Center and Department of Physics, Bar-Ilan University, 52900 Ramat Gan, Israel, IL.

# PART I

## Results about Corporate Ownership Network (CON).

As described in the article, we construct CON by using the ORBIS database. ORBIS contains the 4000 world corporations with the highest turnover, obtained from the Bureau van Dijk Electronic Publishing (BvDEP), and includes all the corporate ownership relations to their 616000 direct or indirect subsidiaries for the year 2007. From this database we create a network that connects 206 countries around the globe, using as links the ownership relations within large companies. If companies listed in country A have subsidiary corporations in country B, there is a link connecting these two countries directed from country A to country B.

The weight of the link, $w_{AB}$, equals the number of the subsidiary corporations in country B controlled by companies of country A. Next, if companies from country B have subsidiary corporations in country C, then again there is a weighted link, $w_{BC}$, connecting these two countries directed from B to C, and so on. This way we obtain a network with total 2886 links among 206 nodes (countries). Of these links 685 are bi-directional, meaning that if there is a link from node *i* to *j*, there is also a link from node *j* to *i*, and the rest 1516 are one directional only.

We assume that the total link weight between a pair of nodes (countries) *ij* is the sum of all links independently of their direction, $w_{tot}^{(ij)} = w_{ij} + w_{ji}$. The total link weight represents the strength of economic ties between two countries in the network. We can quantify the total economic strength of a country *i* by means of the total node weight, $\tilde{w}_{tot}^{i} = \sum_j w_{ij} + \sum_j w_{ji}$ which sums the weights of all links of node *i*.

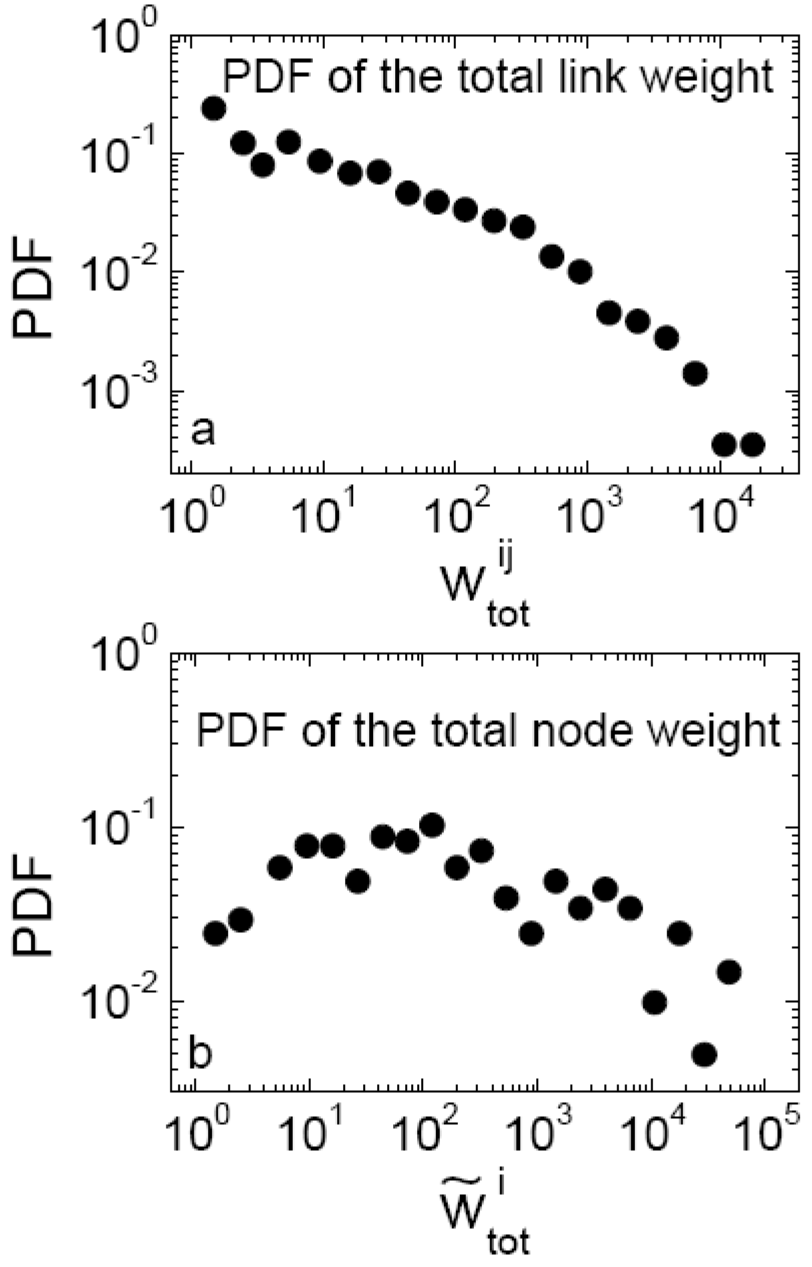


**Supplementary Figure S1**. The probability density distributions of (a) the total node weights and (b) the total link weights. Both are skewed and heavy tailed.

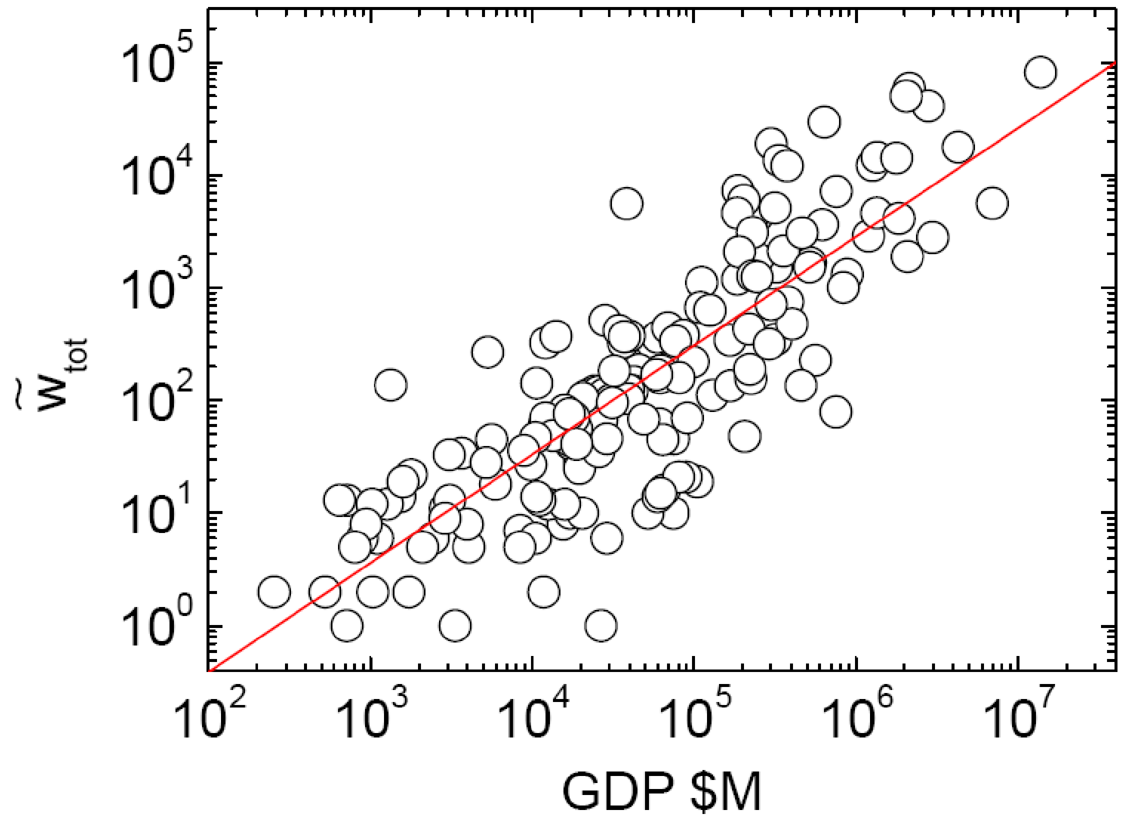


**Supplementary Figure S2**. Scatter plot of the total node weight $\tilde{w}_{tot}^{i} = \sum_j w_{ij} + \sum_j w_{ji}$ of a node *i* versus its actual GDP value obtained from the International Monetary Fund (IMF) for the year 2007. The red line corresponds to the best fit on the data, and has slope 0.96±0.05. The almost linear relation reveals the strong correlation of our measure of strength $\tilde{w}_{tot}^{i}$ and the GDP of the corresponding countries. The strong correlations suggest that our network is a good approximation for the actual economic relations, and the parameters we use in our model have a direct analogy to the real economy.

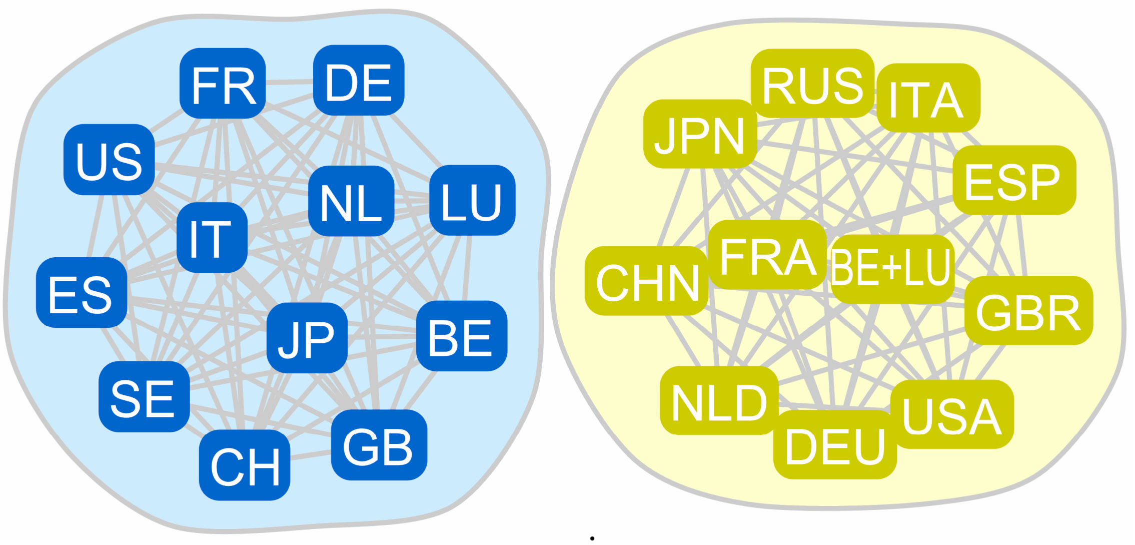


**Supplementary Figure S3**. The strongest connected communities obtained by implementing the Clique Percolation Method [Palla et al. *Nature* **435**:814-818 (2005)] on CON for $w_c \geq 100$ (left), and on the ITN (see next section) for $w_c \geq 5100$ $M (right). These communities are the same with the nuclei we found using the *k*-shell decomposition method.

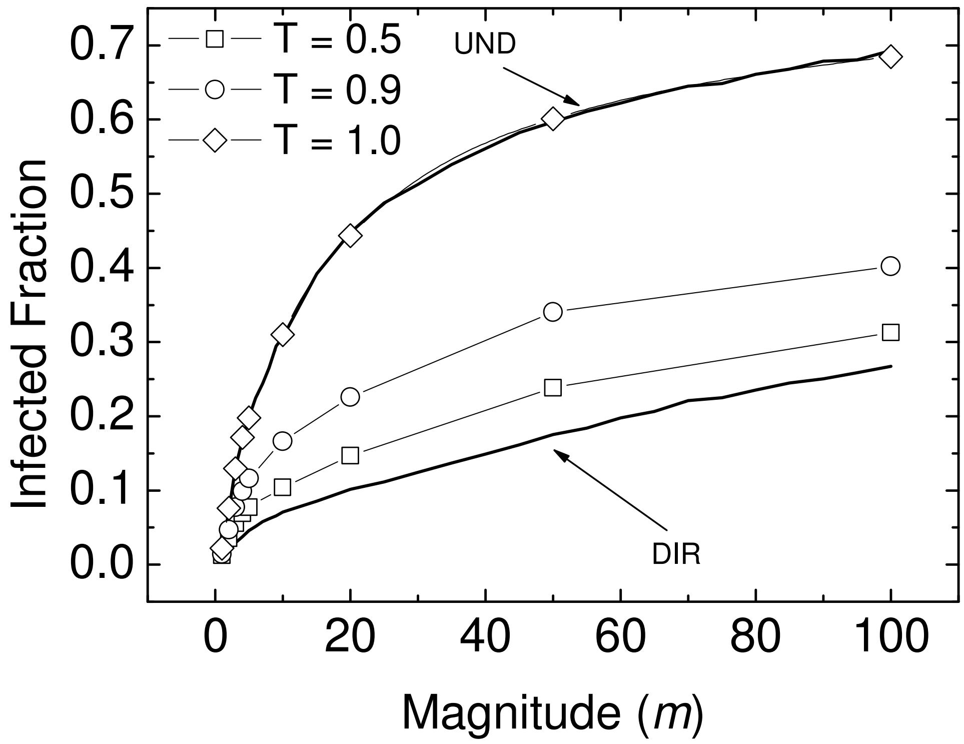


**Supplementary Figure S4**. Fraction of nodes infected by a crisis versus the magnitude *m* of the crisis. The results obtained using different parameter $T$ values, and are averages over 50 realizations for a crisis starting at each node of the network. Note that for low values of T (T<=0.5) the results are not sensitive on T. Further increasing $T$ progressively speeds up the spreading of crises, and as expected, for the limit case, $T=1$, the epidemic spreading is exactly that obtained for the undirected case (UND).

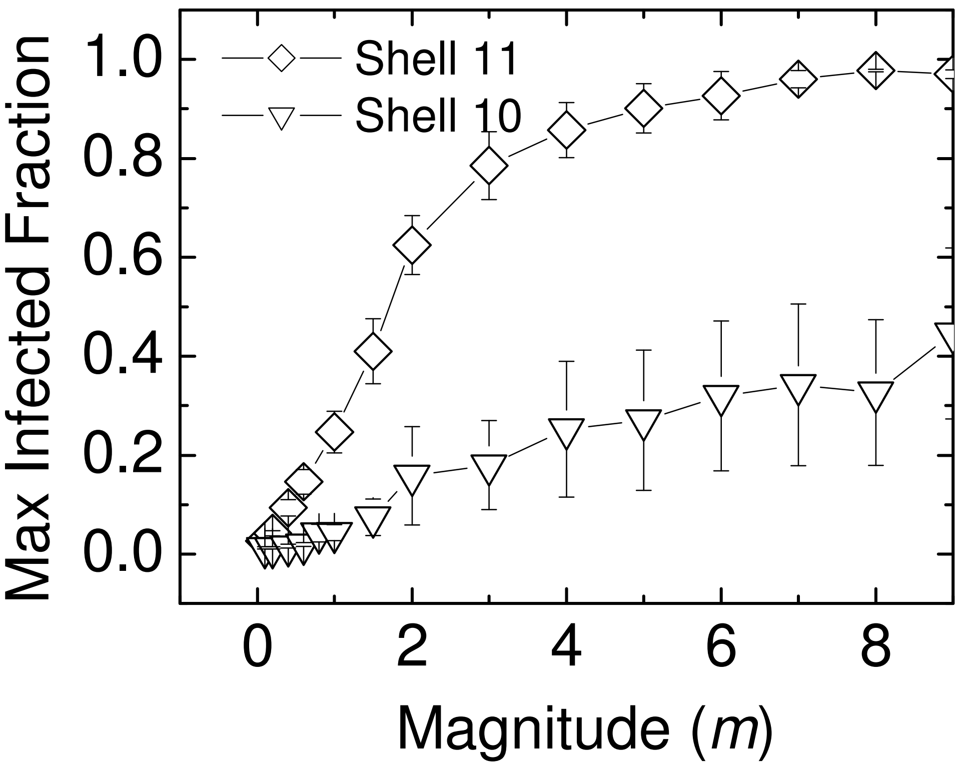


**Supplementary Figure S5**. The maximum fraction of infected nodes versus the crisis magnitude *m.* We can identify a critical *m* values where crisis starts spreading rapidly (we have an epidemic outbreak), e.g. *m* = 2 for shell 11. These *m* values, and the percentage of the infected countries are dependent to the shell the crisis is originated.

# PART II

### Results about the International Trade Network (ITN).

As described in the article, we construct the ITN by using the 2007 version of the CHELEM database obtained by the Bureau van Dijk Electronic Publishing (BvDEP). The database contains detailed information about international trade, and GDP values in million US dollars. For our analysis, we calculated the aggregated trade actions between all pairs of the 82 countries that were included in the database. From the trading relations between pair of countries e.g., A and B, we can create a bi-directional network where the $E_{AB}$ represents the export of A to B, and $E_{BA}$ represents the export of B to A. Of course $E_{AB}$ is equal to $I_{BA}$, where $I_{BA}$ stands for the imports of B from A.

To be consistent with the notation used about CON, we define that $w_{ij} \equiv E_{ij}$. Therefore, the total link weight between a pair of nodes (countries) *ij* is calculated by $w_{tot}^{(ij)} = E_{ij} + E_{ji}$. This is the actual measure of the total trade flow between node *I* and node *j.* Furthermore, we calculate the trade balance (a quantity describing the balance of payment between each pair of countries) as $b = E_{AB} - E_{BA}$. Note that the trade balance is the numerator of Eq. (2) and is the factor that creates the directionality of the network.

In order to study the propagation of crises in the ITN, we applied the SIR model that is described in the manuscript. Similar to the implementation we used for CON, we assume that the probability $p_{ij}$ that node $i$ (a country in crisis) infects node *j* (a country not yet affected) is given by $p_{ij} \propto m \cdot w^{(ij)} / \tilde{w}_{tot}^{j}$. Here, $w^{(ij)}$ is the link weight (representing the total trade) between country $i$ and country $j$ in Million $US and $\tilde{w}_{tot}^{j}$ is the GDP of country $j$.

If the fraction $w^{(ij)} / \tilde{w}_{tot}^{j}$ is large, it means that the economy of country $j$ is strongly affected by the bilateral trade with country $i$. This results to a high probability that country $j$ will be affected by a crisis propagating through its link to country $i$. The factor $m$ represents the strength of the crisis and therefore it can take any positive value.

Figs. S6-S8 show that while the maximum fraction of the infected nodes using the ITN is able to obtain high values for relatively small magnitudes, it does not show any sharp transition like the one shown in Fig. S5 for CON.

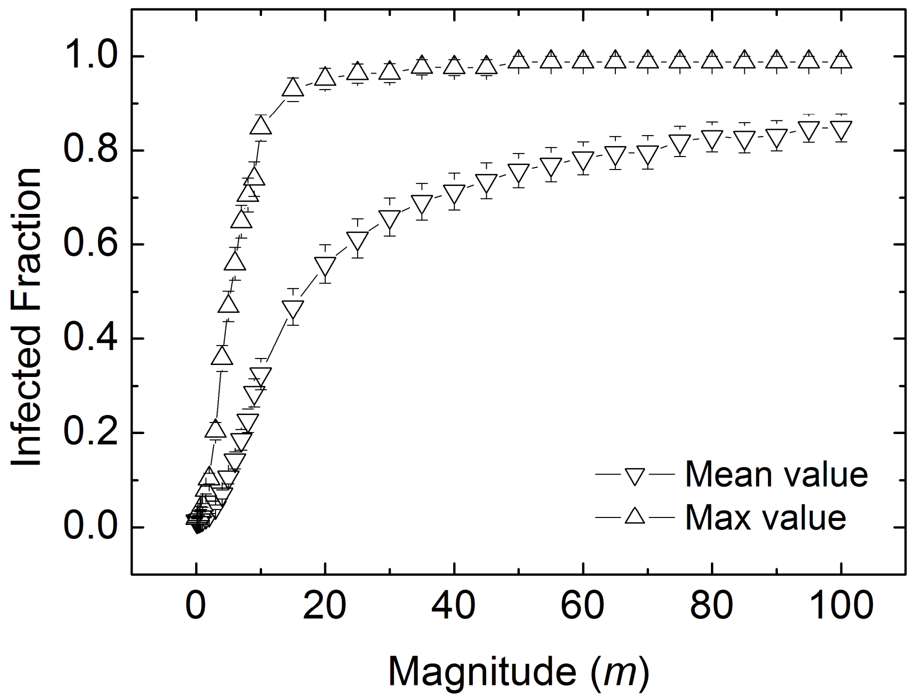


**Supplementary Figure S6**. Fraction of nodes infected and maximum fraction of the infected nodes by a crisis spreading using the SIR model versus the magnitude *m* of the crisis. The results are averages over 50 realizations for a crisis starting at each node of the network, and the error bars are showing the standard deviation.

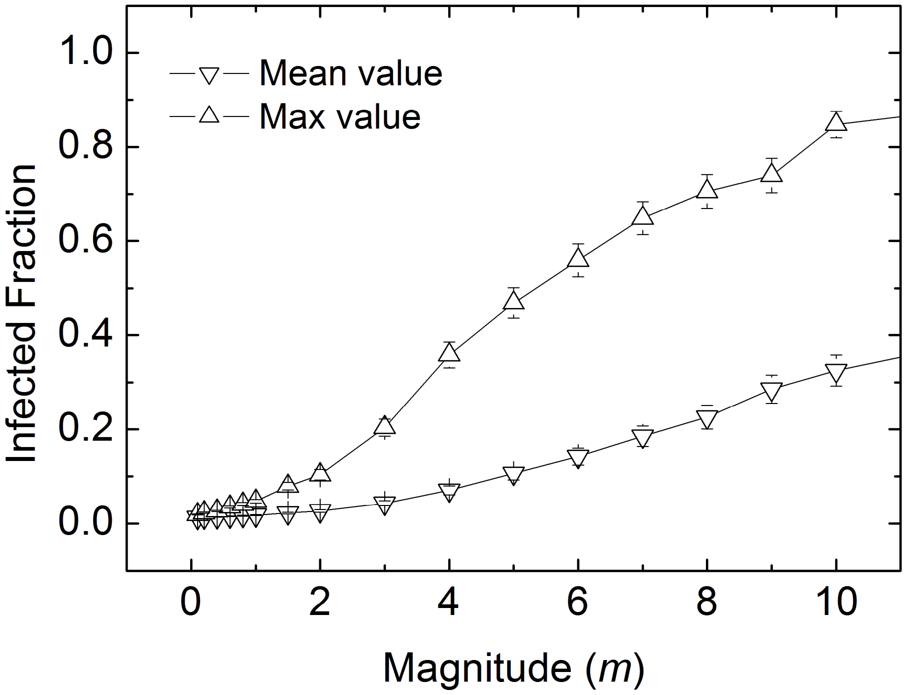


**Supplementary Figure S7**. Zoom of the area showing the spreading for smaller crisis magnitudes *m* of Supplementary Figure S6. The results are averages over 50 realizations for a crisis starting at each node of the network, and the error bars are showing the standard deviation.

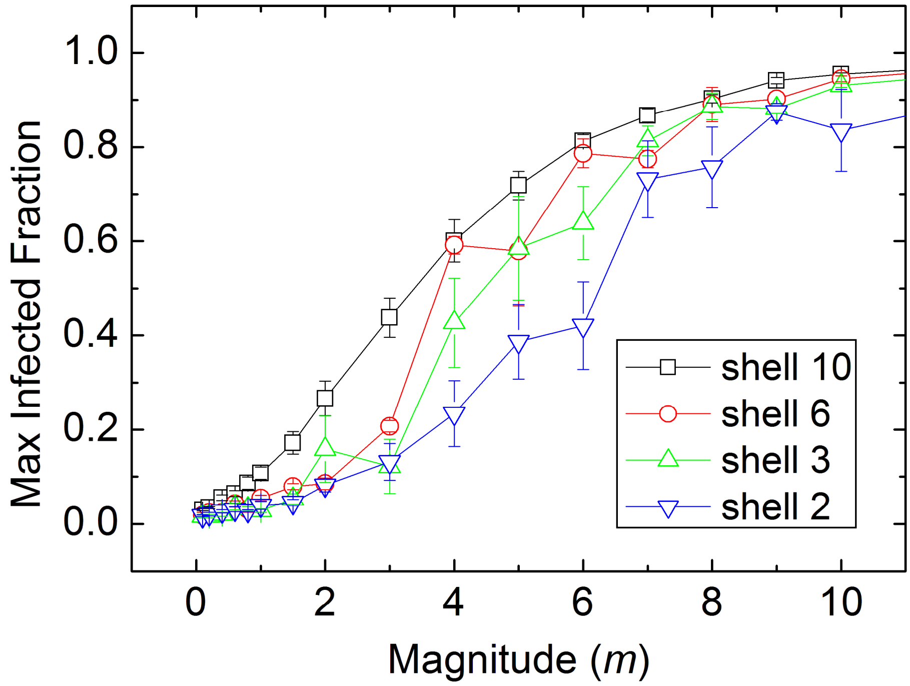


**Supplementary Figure S8**. The maximum fraction of the infected nodes by a crisis originating from different shells of the network versus its magnitude *m.* The results are averages over 50 realizations, and the error bars are showing the standard deviation.

## PART III

### Spreading of a crisis started in Greece.

In this section we used our model to understand into what extent a crisis originating in Greece could spread to other countries. For both networks (CON and ITN) describing economic activity we obtained similar results. Our findings indicate that a large crisis has the potential to propagate to large percentage of the world countries. The worst case scenario, which is given by the maximum value of the infected fraction, shows a rapid global contagion for both networks, stressing that the current situation in Greece needs to be dealt fast and accurately.

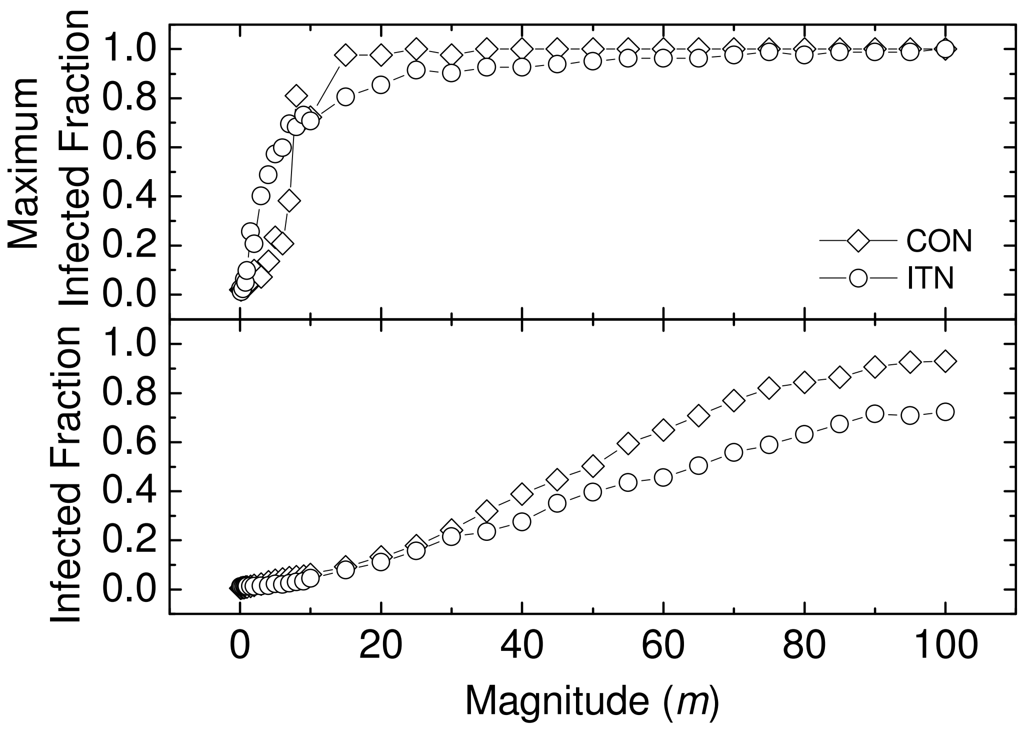


**Supplementary Figure S9**. The fraction of infected countries, and the maximum fraction of infected countries versus the magnitude *m* of a crisis originated in Greece and spread to the rest of the world through CON and ITN. The results are averages over 1000 realizations.

**Supplementary Table S1**. Mean probability of infection of different countries from crises originating in Greece for $m \in [1,100]$.

| | CON | | ITN | | |
|---|---|---|---|---|---|
| Country code | Mean infection probability | Standard deviation | Mean infection probability | Standard deviation | Group |
| AL | 0.97 | 0.17 | 0.2 | 0.40 | **Proximal countries** |
| MK | 0.98 | 0.14 | 0.22 | 0.41 | |
| BA | 0.86 | 0.34 | 0.34 | 0.47 | |
| TR | 0.59 | 0.49 | 0.38 | 0.48 | |
| IL | 0.41 | 0.49 | 0.31 | 0.46 | |
| BG* | 0.90 | 0.30 | 0.44 | 0.49 | |
| RO* | 0.82 | 0.38 | 0.38 | 0.48 | |
| PT | 0.45 | 0.50 | 0.38 | 0.48 | **EU members** [*BG and RO are EU members as well] |
| AU | 0.41 | 0.49 | 0.38 | 0.48 | |
| BE | 0.40 | 0.49 | 0.38 | 0.48 | |
| DE | 0.40 | 0.49 | 0.38 | 0.48 | |
| DK | 0.40 | 0.49 | 0.37 | 0.48 | |
| ES | 0.40 | 0.49 | 0.38 | 0.48 | |
| FI | 0.40 | 0.49 | 0.38 | 0.48 | |
| GB | 0.40 | 0.49 | 0.38 | 0.48 | |
| IT | 0.40 | 0.49 | 0.38 | 0.48 | |
| LU | 0.40 | 0.49 | 0.38 | 0.48 | |
| NL | 0.40 | 0.49 | 0.38 | 0.48 | |
| IE | 0.44 | 0.49 | 0.38 | 0.48 | |
| US | 0.40 | 0.49 | 0.38 | 0.48 | **Other large economies** |
| JP | 0.40 | 0.49 | 0.38 | 0.48 | |
| CA | 0.43 | 0.49 | 0.38 | 0.48 | |
| CN | 0.52 | 0.50 | 0.38 | 0.48 | |
| RU | 0.62 | 0.48 | 0.38 | 0.48 | |

As it is presented here, CON is more sensitive in comparison to the ITN, and it predicts an easier propagation of a crisis to countries in the neighbour of Greece (South-Eastern Europe). These countries traditionally have strong economic ties with Greece.
